# Supplementary material for: Closeness Centrality Algorithms For Multilayer Networks
Source: arXiv:2207.11662 source file (2023-08-13)
Supplement: Supplementary file 1 [file Appendices.tex]

\section{Appendix}
\label{sec:appendix}
\appendix

%%\textbf{Algorithm for Closeness Centrality Heuristic 1}

%%\textbf{Algorithm for Closeness Centrality Heuristic 2}
