# Supplementary material for: Closeness Centrality Algorithms For Multilayer Networks
Source: arXiv:2207.11662 source file (2023-08-13)
Supplement: Supplementary file 2 [file Appendix_old.tex]

\section{Appendix}
\label{sec:appendix}

This appendix explains the steps to create synthetic datasets using RMAT, setting up the environment in the SDSC expanse, and running the experiments.

\subsection{Creating and Preprocessing Synthetic Datasets}

The synthetic datasets are generated using RMAT. We use a fork of RMAT called PaRMAT with multithreading support. \href{https://github.com/farkhor/PaRMAT}{This} is the link to the git repository containing PaRMAT. The repository link contains detailed instructions to set up and run the program. The output file generated by PaRMAT contains the edge list of the graph. Each line of the file contains an edge with source vertex and destination vertex separated by a comma. As this format is separate from the format we are using to feed graphs to our algorithms, we have a conversion script that converts the RMAT generated file to our standard format. This python script is the \textit{rmat\textunderscore to\textunderscore networkx.py} script. The script takes four parameters. They are:

i. Number of nodes per layer: How many nodes are in each layer of the network. As RMAT generates an edge list, any disjoint vertex will be ignored and will not be in the RMAT output file. As a reason, our script requires the number of nodes in each layer to add them to the standard format graph output file.


ii. Path to the network: The directory containing the layers generated by RMAT. All the files in the directory will be treated as a layer generated by RMAT and converted to the standard format.

iii. output path: Where the output layers of the network will be written. For each network, two sets of network output are written. One is the RMAT generated network converted to the standard format. The other one is a network where a path graph is overlayed on top of the original layers to create a network where each layer has a single connected component.  

iv. logfile: Contains a summary of the processed layers.
